# Supplementary material for: On the Generalization of Training-based ChatGPT Detection Methods
Source: arXiv:2310.01307 source file (2023-10-03)
Supplement: Supplementary file 1 [file appendix.tex]

\appendix

\section{Prompt Design}

Review (IMDb):
\begin{itemize}
    \item  \textit{P1:} ``Write a review for $<$MovieTitle$>$  in [\gray{50, 100, 200}] words''. 
    \item \textit{P2:} ``Develop an engaging and creative review for $<$MovieTitle$>$ in [\gray{50, 100, 200}] words. Follow the writing style of the movie comments as in popular movie review websites such as imdb.com. 
    \item \textit{P3:} ``Complete the following: I just watched $<$MovieTitle$>$. It is [\gray{enjoyable, just OK, mediocre, unpleasant, great}]. [\gray{It is because that, The reason is that, I just feel that, I am feeling that}]''. Each gray word in the list has the same chance to be randomly selected. 
\end{itemize}

Writing:
\begin{itemize}
    \item Write a [\gray{200, 300}] words essay with the following title: $<$Title$>$. Do not include the title.
    \item Write a [\gray{200, 300}] words essay like a high school student with the following title: $<$Title$>$. Do not include the title.
    \item Write a [\gray{200, 300}] words essay like a novelist with the following title: $<$Title$>$. Do not include the title.
\end{itemize}

News:
\begin{itemize}
    \item Write a [\gray{150, 300}] words article like a journalist following the summary: $<$Summary$>$
    \item Write a [\gray{150, 300}] words article following the summary: $<$Summary$>$
    \item Write a [\gray{150, 300}] words article like a commentator following the summary: $<$Summary$>$
\end{itemize}

Question Answering: 
\begin{itemize}
    \item \textit{P1:} ``Answer the following question in no more than $<$\gray{50, 100, 150}$>$ words:$<$Question$>$'' 
    \item \textit{P3:} ``Act as if you are a user in Reddit or Quora, answer the following question in no more than $<$\gray{50, 100, 150}$>$ words. $<$Question$>$'' Do not include user id in the answer.'' 
    \item \textit{P2:} P1 + ``Please explain like I'm five.'' 
\end{itemize}

\section{More Result about Prompts}

\begin{figure}

\vspace{0.2cm}
\subfloat[\footnotesize News]
{\label{fig:ad2}
\begin{minipage}[b]{0.24\linewidth}
\centering
\includegraphics[width=1.2\textwidth]{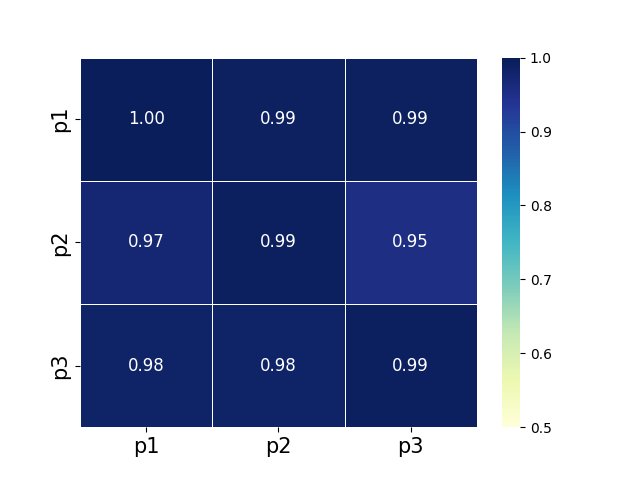}
\end{minipage}
}
\subfloat[\footnotesize Review]{\label{fig:ad1}
\begin{minipage}[b]{0.24\linewidth}
\centering
\includegraphics[width=1.2\textwidth]{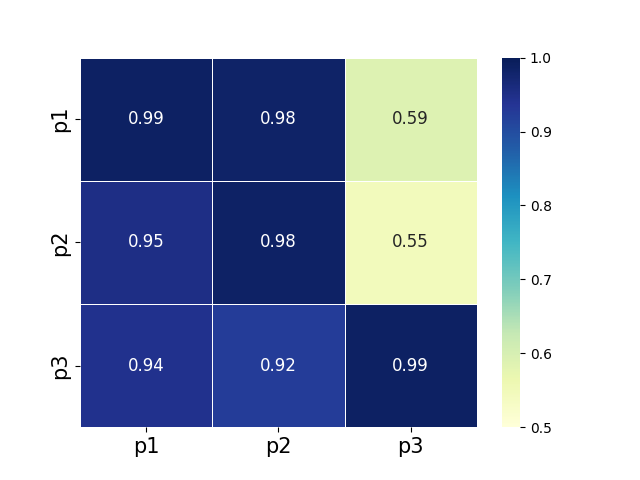}
\end{minipage}
}
\subfloat[\footnotesize Writing]
{\label{fig:ad2}
\begin{minipage}[b]{0.24\linewidth}
\centering
\includegraphics[width=1.2\textwidth]{figures/pp3.png}
\end{minipage}
}
\subfloat[\footnotesize QA]
{\label{fig:ad3}
\begin{minipage}[b]{0.24\linewidth}
\centering
\includegraphics[width=1.2\textwidth]{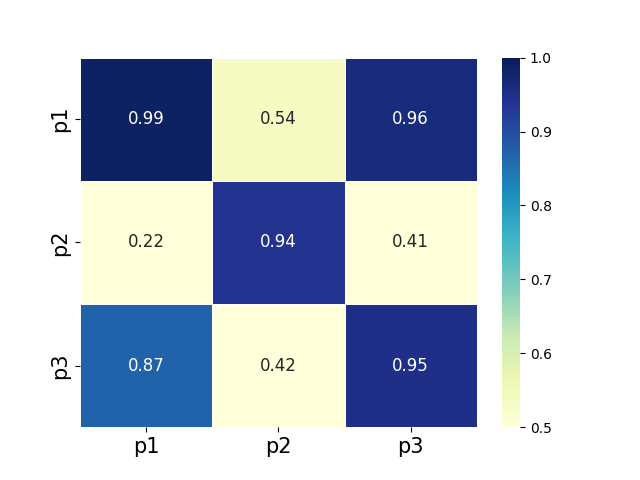}
\end{minipage}
}
\caption{\small Prompt Generalization for GPT-PAT}
\label{fig:rare_benefit}
\end{figure}

The impact of prompts in training, evaluated on diverse prompts. (GLTR, RoBERTa-base, RoBERTa-large, T-5, MPU, GPT-Pat)
\begin{figure}[h]
\subfloat[\footnotesize News \red{(TODO)}]
{\label{fig:ad2}
\begin{minipage}[b]{0.24\linewidth}
\centering
\includegraphics[width=1.1\textwidth]{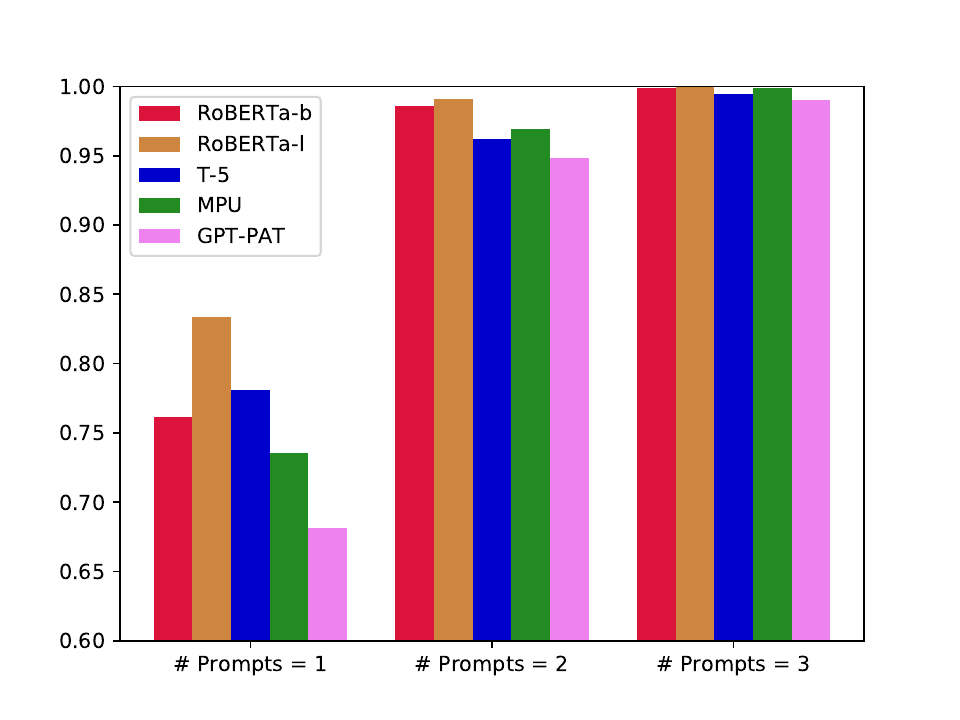}
\end{minipage}
}
\subfloat[\footnotesize Review]{\label{fig:ad1}
\begin{minipage}[b]{0.24\linewidth}
\centering
\includegraphics[width=1.1\textwidth]{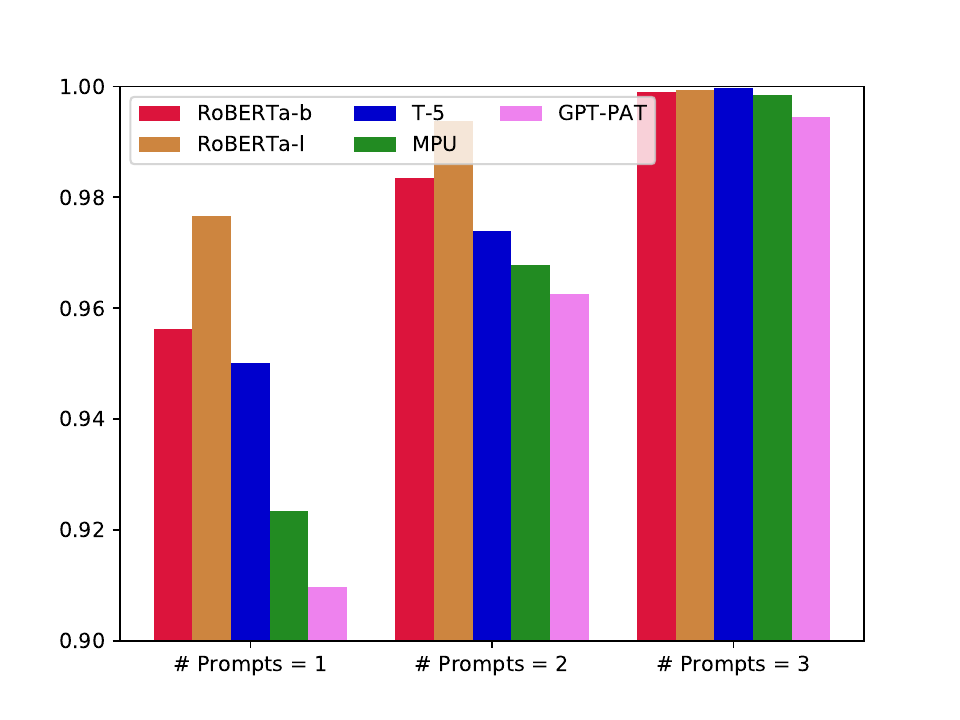}
\end{minipage}
}
\subfloat[\footnotesize Writing]
{\label{fig:ad2}
\begin{minipage}[b]{0.24\linewidth}
\centering
\includegraphics[width=1.1\textwidth]{figures/ivypanda_random_prompt.pdf}
\end{minipage}
}
\subfloat[\footnotesize QA]
{\label{fig:ad3}
\begin{minipage}[b]{0.24\linewidth}
\centering
\includegraphics[width=1.1\textwidth]{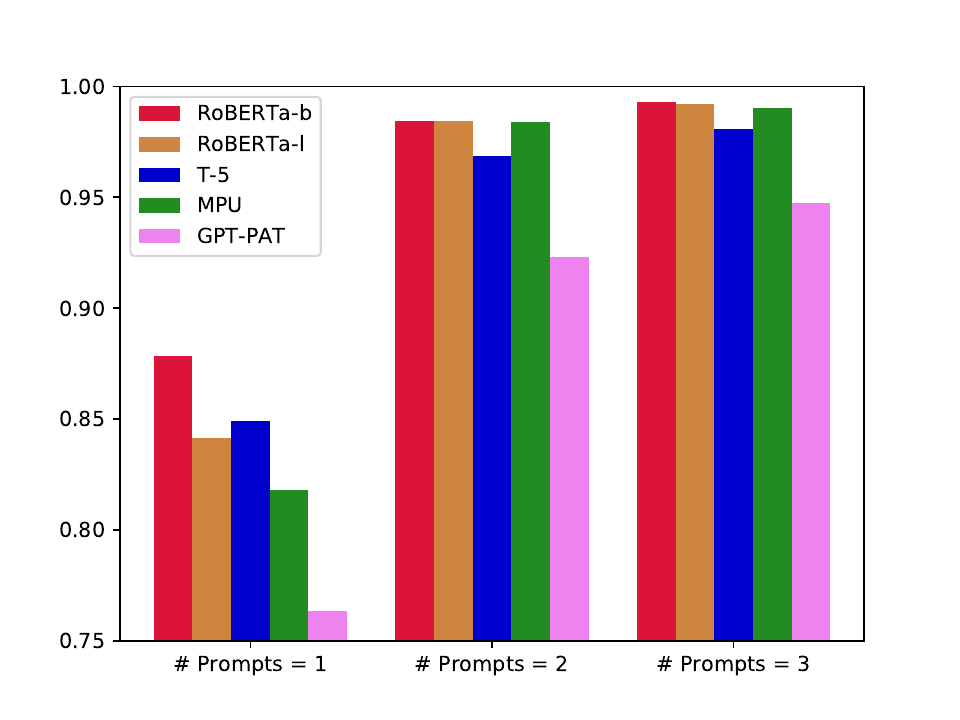}
\end{minipage}
}
\caption{\small 123123123}
\label{fig:rare_benefit}
\end{figure}

\begin{figure}[h!]
\subfloat[\footnotesize AUROC]{\label{fig:ad1}
\begin{minipage}[b]{0.23\linewidth}
\centering
\includegraphics[width=1.1\textwidth]{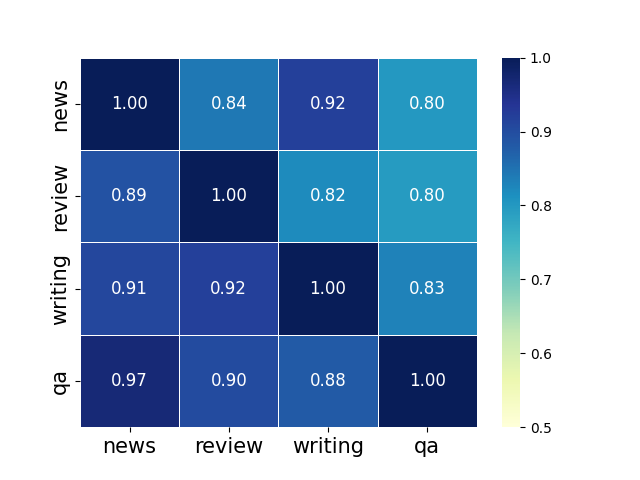}
\end{minipage}
}
\subfloat[\footnotesize F1 Score]
{\label{fig:ad2}
\begin{minipage}[b]{0.23\linewidth}
\centering
\includegraphics[width=1.1\textwidth]{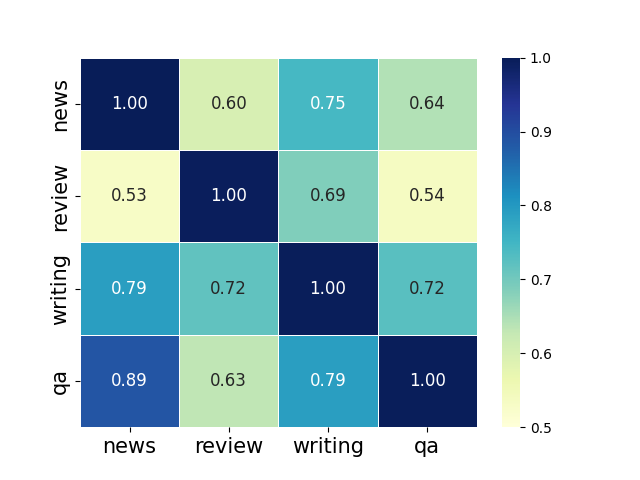}
\end{minipage}
}
\subfloat[\footnotesize TPR]
{\label{fig:ad3}
\begin{minipage}[b]{0.23\linewidth}
\centering
\includegraphics[width=1.1\textwidth]{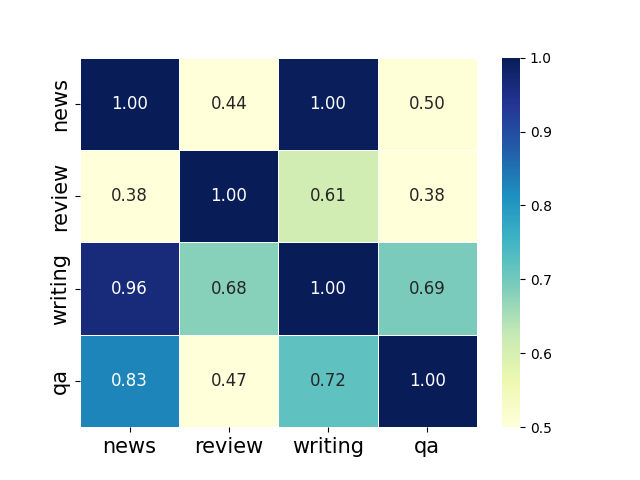}
\end{minipage}
}
\subfloat[\footnotesize 1-FPR]
{\label{fig:ad4}
\begin{minipage}[b]{0.23\linewidth}
\centering
\includegraphics[width=1.1\textwidth]{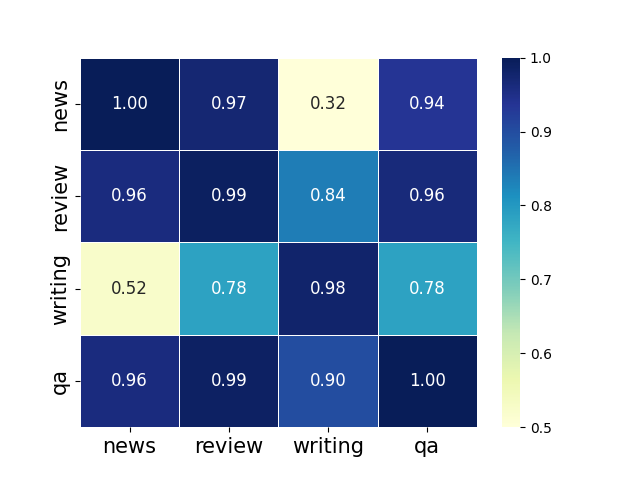}
\end{minipage}
}
\caption{\small Domain-wise Generalization of GPT-Pat Detection}
\label{fig:transfer_roberta}
\end{figure}

\begin{figure}
% \begin{figure}[h!]
\subfloat[\footnotesize AUROC]{\label{fig:ad1}
\begin{minipage}[b]{0.23\linewidth}
\centering
\includegraphics[width=1.1\textwidth]{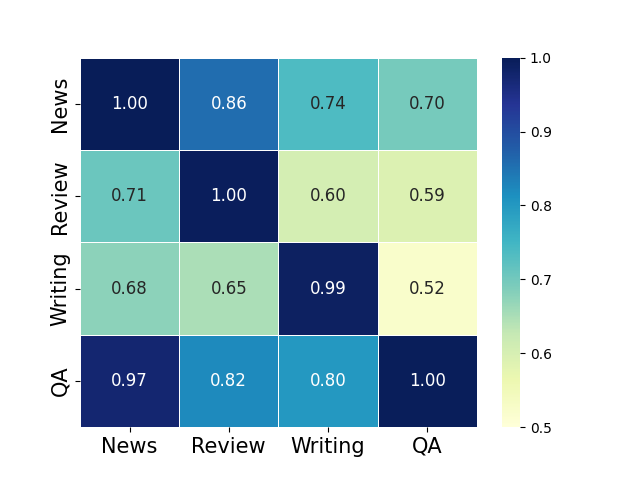}
\end{minipage}
}
\subfloat[\footnotesize F1 Score]
{\label{fig:ad2}
\begin{minipage}[b]{0.23\linewidth}
\centering
\includegraphics[width=1.1\textwidth]{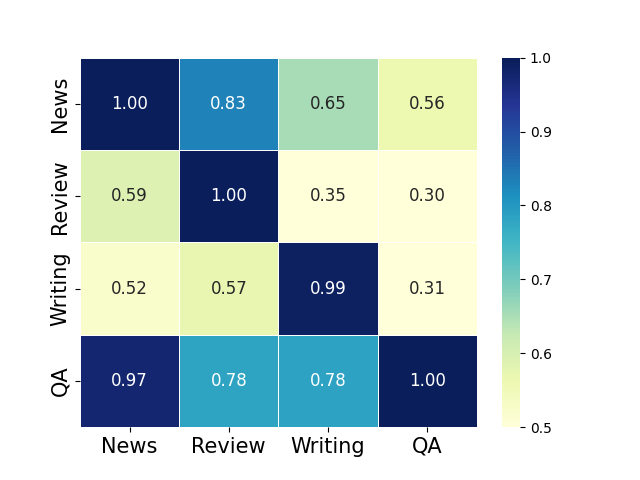}
\end{minipage}
}
\subfloat[\footnotesize TPR]
{\label{fig:ad3}
\begin{minipage}[b]{0.23\linewidth}
\centering
\includegraphics[width=1.1\textwidth]{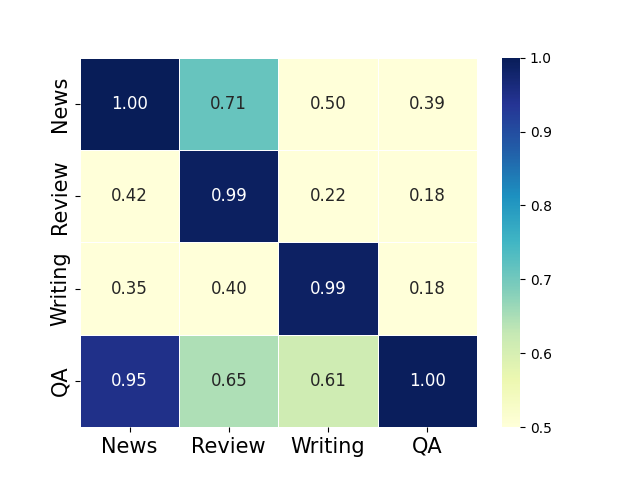}
\end{minipage}
}
\subfloat[\footnotesize 1-FPR]
{\label{fig:ad4}
\begin{minipage}[b]{0.23\linewidth}
\centering
\includegraphics[width=1.1\textwidth]{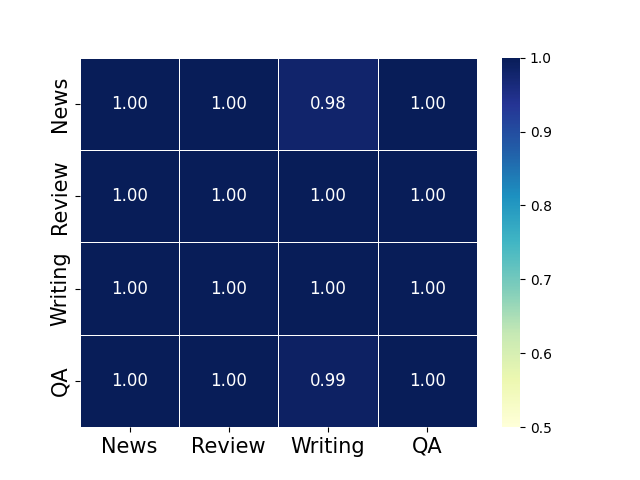}
\end{minipage}
}
\caption{\small Domain-wise Generalization of RoBERTa-base Detection \textbf{with Human Augmentation}}
\label{fig:transfer_ttt}
\end{figure}

\begin{figure}
%%%%%%
\subfloat[\footnotesize News]
{\label{fig:ad2}
\begin{minipage}[b]{0.24\linewidth}
\centering
\includegraphics[width=1.1\textwidth]{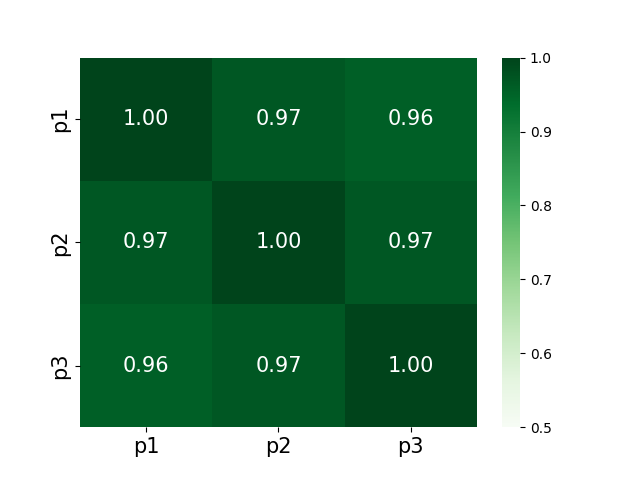}
\end{minipage}
}
\subfloat[\footnotesize Review]{\label{fig:ad1}
\begin{minipage}[b]{0.24\linewidth}
\centering
\includegraphics[width=1.1\textwidth]{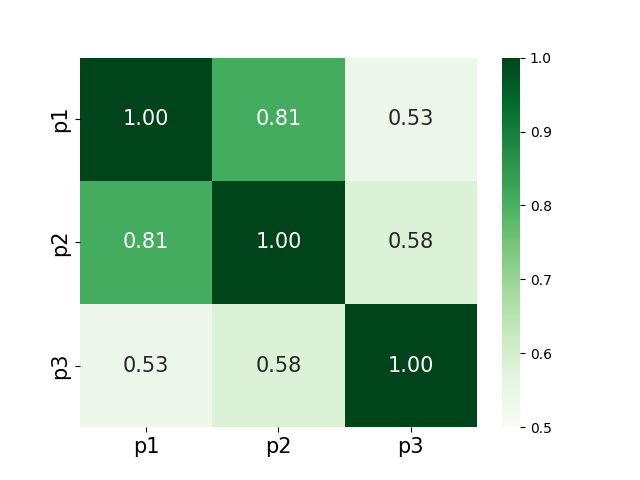}
\end{minipage}
}
\subfloat[\footnotesize Writing]
{\label{fig:ad2}
\begin{minipage}[b]{0.24\linewidth}
\centering
\includegraphics[width=1.1\textwidth]{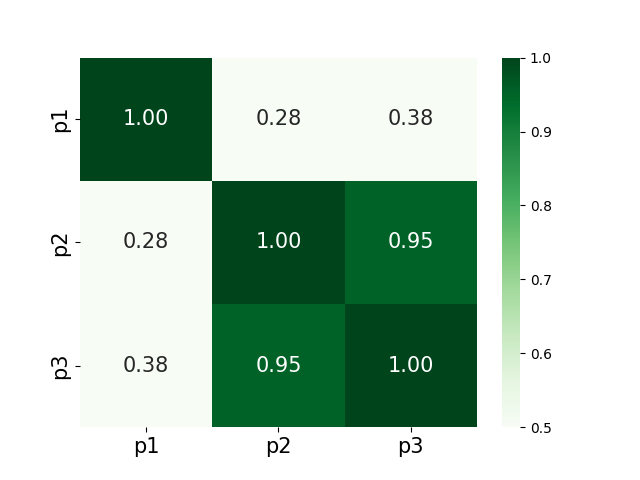}
\end{minipage}
}
\subfloat[\footnotesize QA]
{\label{fig:ad3}
\begin{minipage}[b]{0.24\linewidth}
\centering
\includegraphics[width=1.1\textwidth]{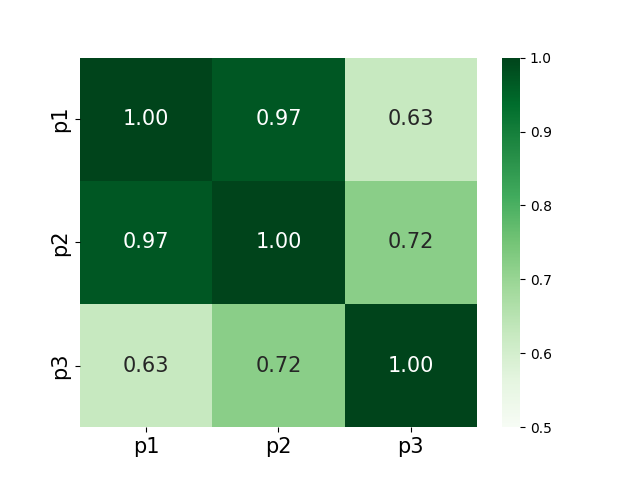}
\end{minipage}
}
\caption{\small MAUVE Similarity between ChatGPT Texts among Different Prompts}
\label{fig:rare_similar}
\end{figure}

\begin{figure}[h]
\subfloat[\footnotesize News]
{\label{fig:ad2}
\begin{minipage}[b]{0.24\linewidth}
\centering
\includegraphics[width=1.1\textwidth]{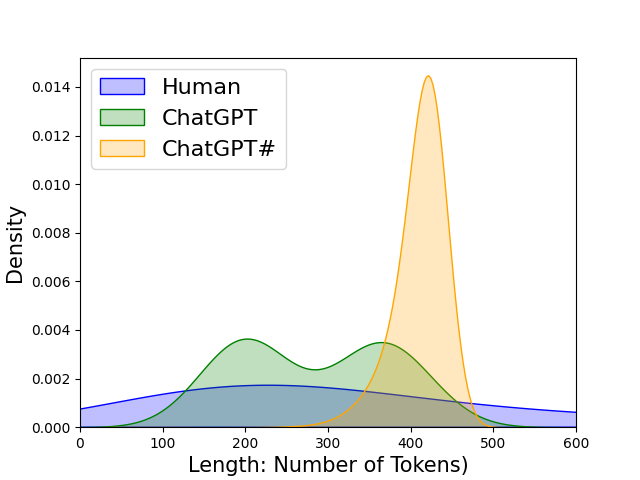}
\end{minipage}
}
\subfloat[\footnotesize Review]{\label{fig:ad1}
\begin{minipage}[b]{0.24\linewidth}
\centering
\includegraphics[width=1.1\textwidth]{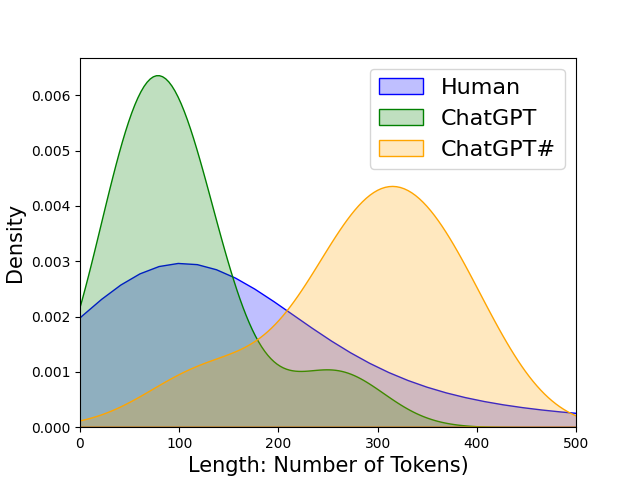}
\end{minipage}
}
\subfloat[\footnotesize Writing]
{\label{fig:ad2}
\begin{minipage}[b]{0.24\linewidth}
\centering
\includegraphics[width=1.1\textwidth]{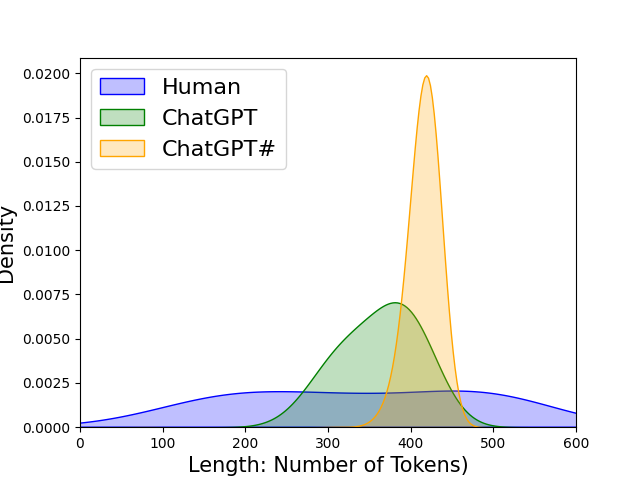}
\end{minipage}
}
\subfloat[\footnotesize QA]
{\label{fig:ad3}
\begin{minipage}[b]{0.24\linewidth}
\centering
\includegraphics[width=1.1\textwidth]{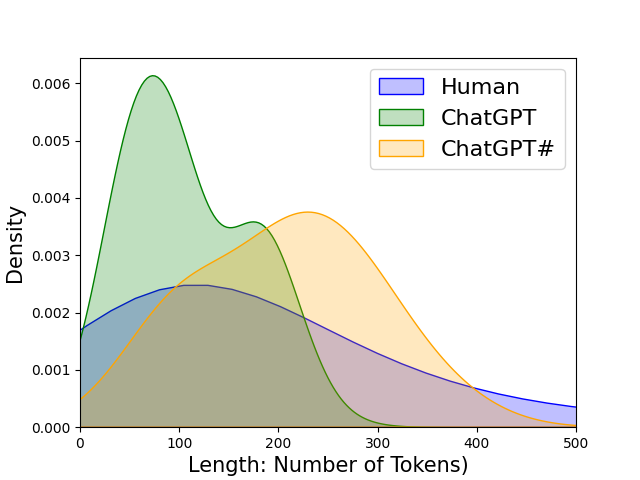}
\end{minipage}
}
\caption{\small Distribution of Length of Human / ChatGPT Texts}
\label{fig:rare_benefit}
\subfloat[\footnotesize News]
{\label{fig:ad2}
\begin{minipage}[b]{0.24\linewidth}
\centering
\includegraphics[height=3cm]{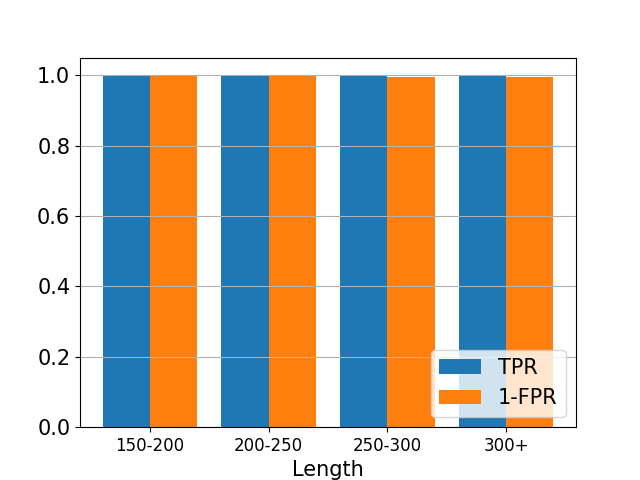}
\end{minipage}
}
\subfloat[\footnotesize Review]{\label{fig:ad1}
\begin{minipage}[b]{0.24\linewidth}
\centering
\includegraphics[height=3cm]{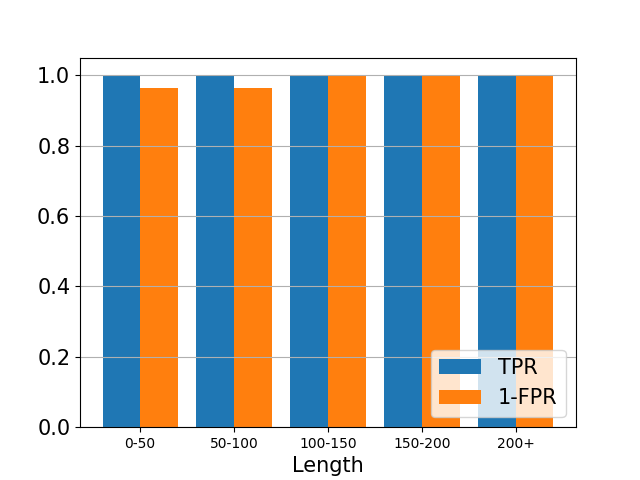}
\end{minipage}
}
\subfloat[\footnotesize Writing]
{\label{fig:ad2}
\begin{minipage}[b]{0.24\linewidth}
\centering
\includegraphics[height=3cm]{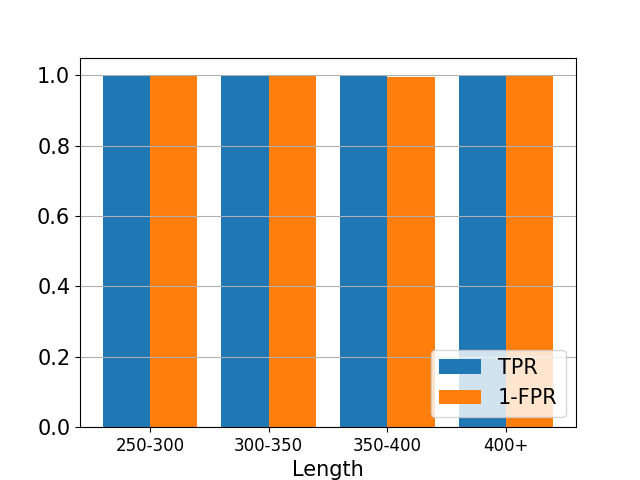}
\end{minipage}
}
\subfloat[\footnotesize QA]
{\label{fig:ad3}
\begin{minipage}[b]{0.24\linewidth}
\centering
\includegraphics[height=3cm]{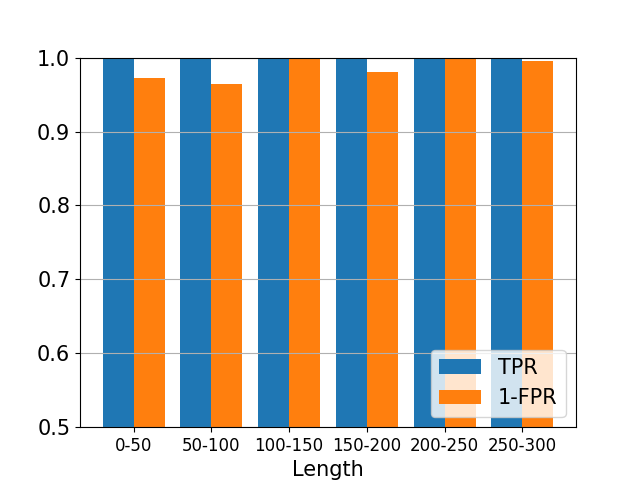}
\end{minipage}
}
\caption{\small Training with Ours}
\label{fig:rare_benefit}
%%%
\subfloat[\footnotesize News]
{\label{fig:ad2}
\begin{minipage}[b]{0.24\linewidth}
\centering
\includegraphics[height=3cm]{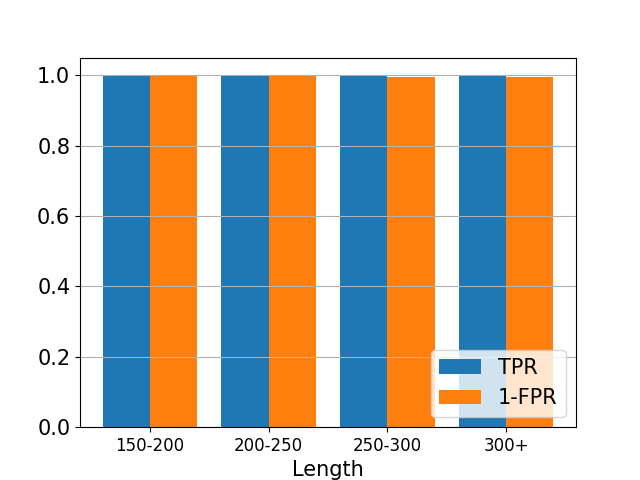}
\end{minipage}
}
\subfloat[\footnotesize Review]{\label{fig:ad1}
\begin{minipage}[b]{0.24\linewidth}
\centering
\includegraphics[height=3cm]{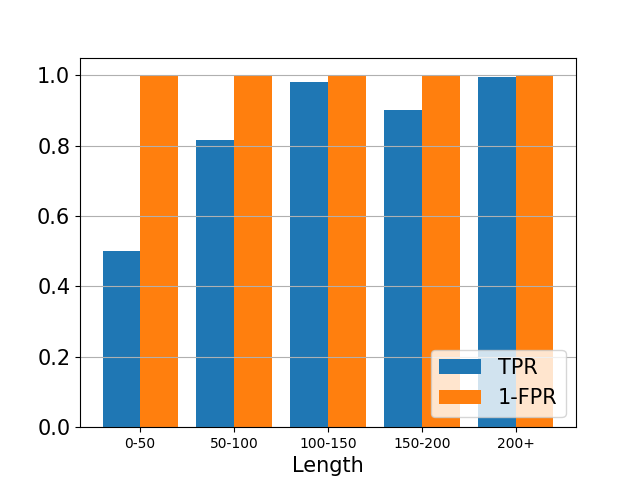}
\end{minipage}
}
\subfloat[\footnotesize Writing]
{\label{fig:ad2}
\begin{minipage}[b]{0.24\linewidth}
\centering
\includegraphics[height=3cm]{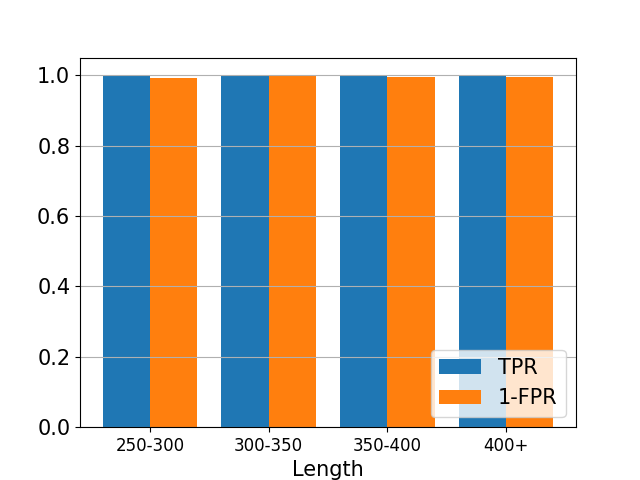}
\end{minipage}
}
\subfloat[\footnotesize QA]
{\label{fig:ad3}
\begin{minipage}[b]{0.24\linewidth}
\centering
\includegraphics[height=3cm]{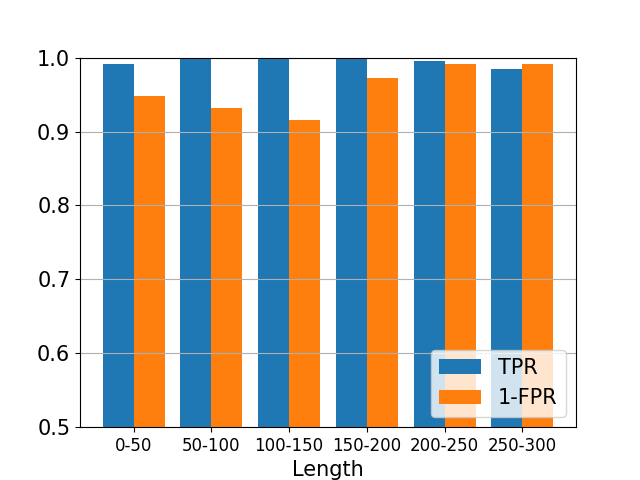}
\end{minipage}
}
\caption{\small Training with ChatGPT Texts without Designating Lengths}
\label{fig:rare_benefit}
\end{figure}

\subsection{Diversity Enhance Generalization}

\begin{wrapfigure}{r}{0.6\textwidth}
\centering
\subfloat[\small Topic-wise Vis. (in QA)]{\label{fig:ad2}
\begin{minipage}[c]{0.3\textwidth}
\centering
\includegraphics[width = 1\textwidth]{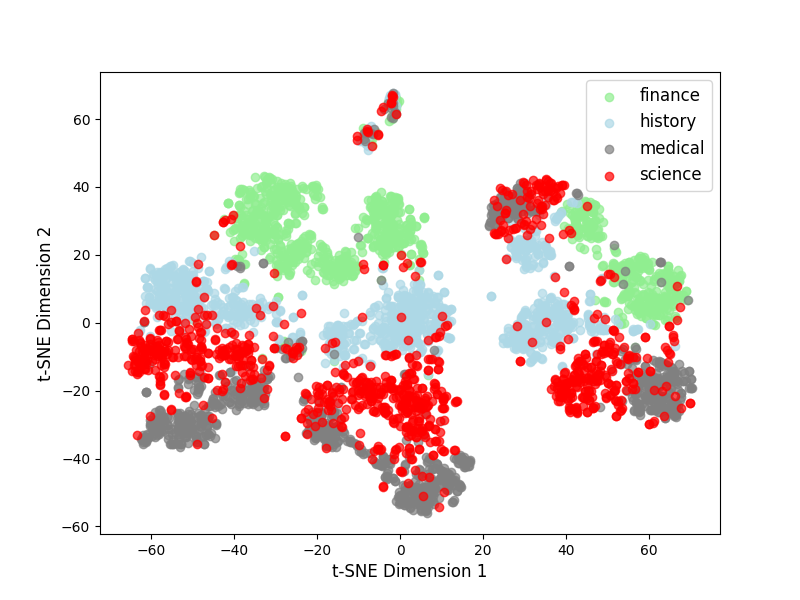}
\end{minipage}
}
\subfloat[\small Domain-wise Vis.]{\label{fig:ad1}
\begin{minipage}[c]{0.3\textwidth}
\centering
\includegraphics[width = 1\textwidth]{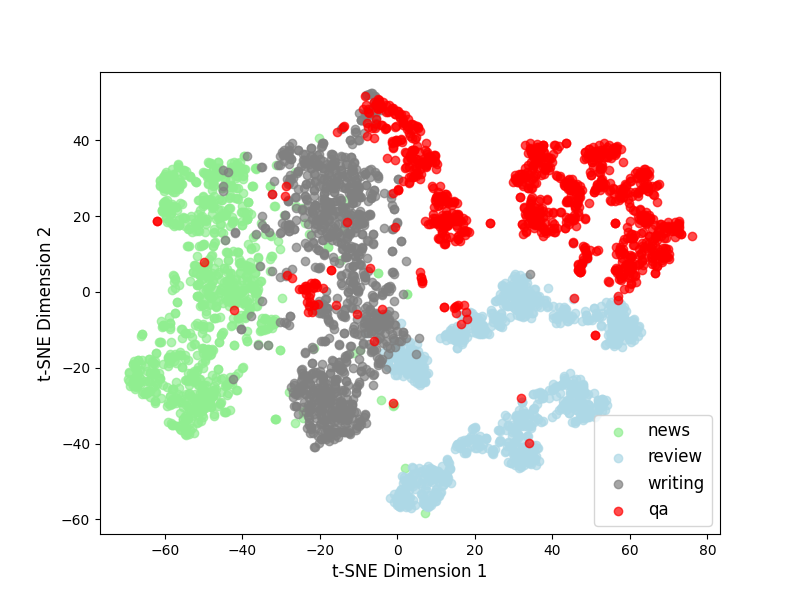}
\end{minipage}
}
\caption{\small Visualization of Last-layer Representation}
\label{fig:landscape}
\end{wrapfigure}
\gray{The abstract paragraph should be indented 1/2~inch (3~picas) on both left and
right-hand margins. Use 10~point type, with a vertical spacing of 11~points.
The word \textsc{Abstract} must be centered, in small caps, and in point size 12. Two
line spaces precede the abstract. The abstract must be limited to one
paragraph.The abstract paragraph should be indented 1/2~inch (3~picas) on both left and
right-hand margins. Use 10~point type, with a vertical spacing of 11~points.
The word \textsc{Abstract} must be centered, in small caps, and in point size 12. Two
line spaces precede the abstract. The abstract must be limited to one
paragraph.The abstract paragraph should be indented 1/2~inch (3~picas) on both left and
right-hand margins. Use 10~point type, with a vertical spacing of 11~points.
The word \textsc{Abstract} must be centered, in small caps, and in point size 12. Two
line spaces precede the abstract. The abstract must be limited to one
paragraph.The abstract paragraph should be indented 1/2~inch (3~picas) on both left and
right-hand margins. Use 10~point type, with a vertical spacing of 11~points.
The word \textsc{Abstract} must be centered, in small caps, and in point size 12. Two
line spaces precede the abstract. The abstract must be limited to one
paragraph.}

\begin{figure}[t]
% \subfloat[\footnotesize AUROC]
% {\label{fig:ad2}
% \begin{minipage}[b]{0.24\linewidth}
% \centering
% \includegraphics[width=1.2\textwidth]{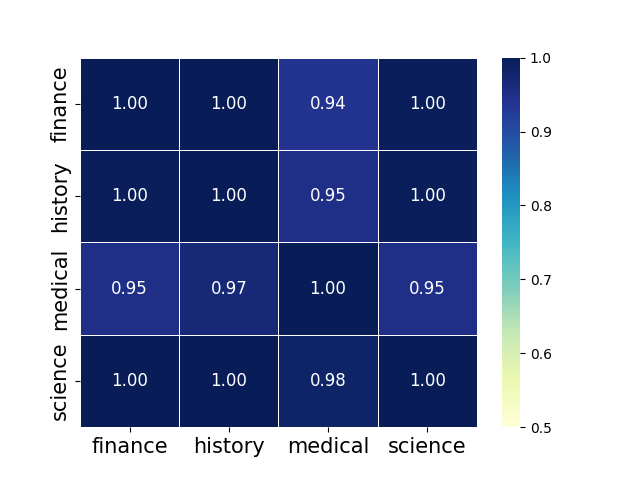}
% \end{minipage}
% }
\centering
\subfloat[\footnotesize AUROC]
{\label{fig:ad2}
\begin{minipage}[b]{0.24\linewidth}
\centering
\includegraphics[width=1.2\textwidth]{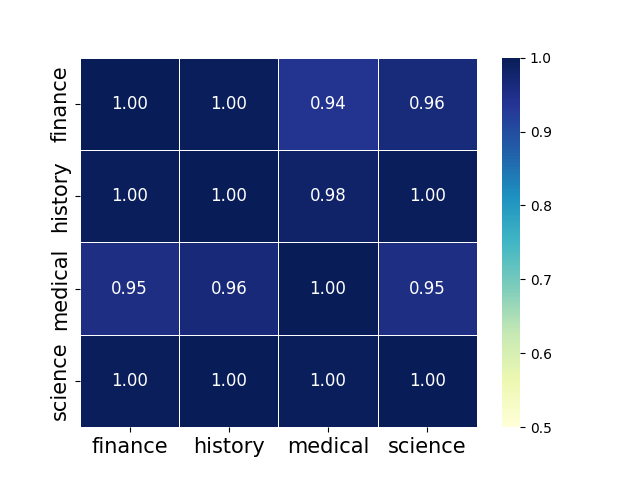}
\end{minipage}
}
\centering
\subfloat[\footnotesize F1 Score]{\label{fig:ad1}
\begin{minipage}[b]{0.24\linewidth}
\centering
\includegraphics[width=1.2\textwidth]{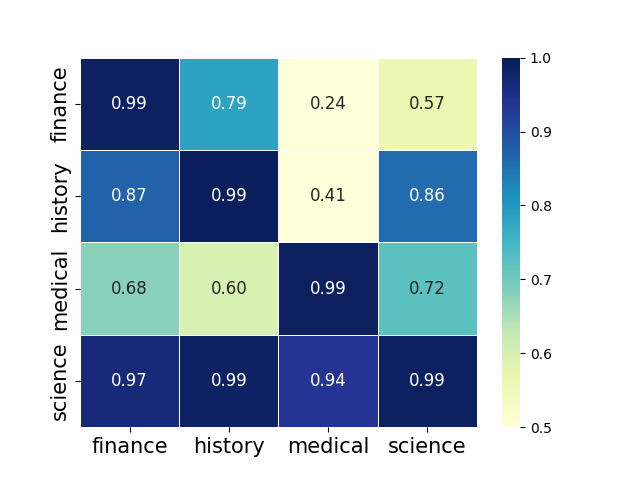}
\end{minipage}
}
\subfloat[\footnotesize TPR]
{\label{fig:ad2}
\begin{minipage}[b]{0.24\linewidth}
\centering
\includegraphics[width=1.2\textwidth]{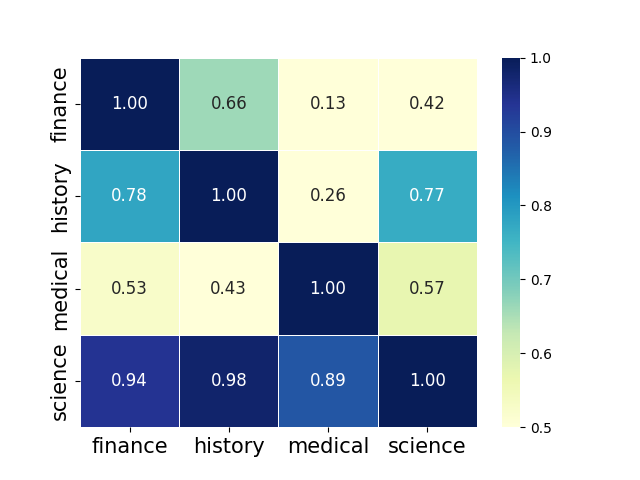}
\end{minipage}
}
\subfloat[\footnotesize 1 - FPR]
{\label{fig:ad3}
\begin{minipage}[b]{0.24\linewidth}
\centering
\includegraphics[width=1.2\textwidth]{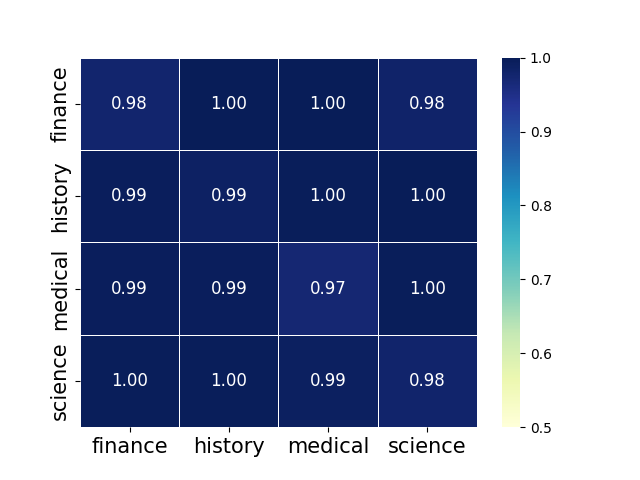}
\end{minipage}
}
\caption{\small Generalization \& MAUVE across Various Topics in QA with all Human Answers}
\label{fig:topic_similar2}
%%%
\subfloat[\footnotesize AUROC]
{\label{fig:ad2}
\begin{minipage}[b]{0.24\linewidth}
\centering
\includegraphics[width=1.2\textwidth]{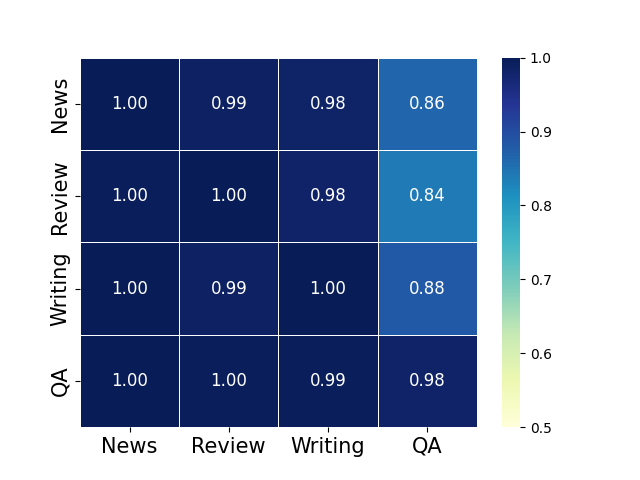}
\end{minipage}
}
\subfloat[\footnotesize F1 Score]{\label{fig:ad1}
\begin{minipage}[b]{0.24\linewidth}
\centering
\includegraphics[width=1.1\textwidth]{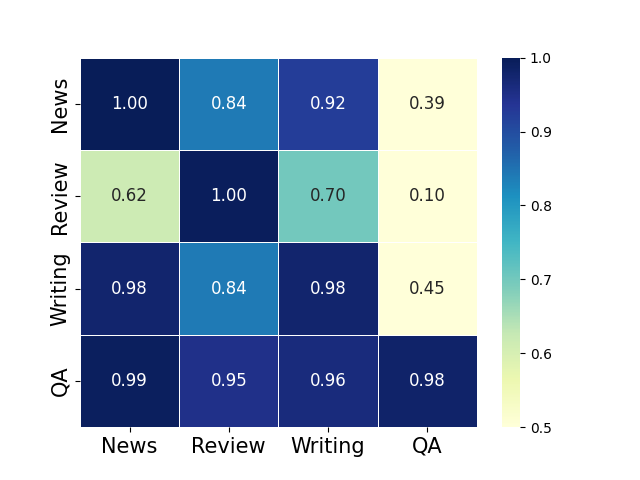}
\end{minipage}
}
\subfloat[\footnotesize TPR]
{\label{fig:ad2}
\begin{minipage}[b]{0.24\linewidth}
\centering
\includegraphics[width=1.1\textwidth]{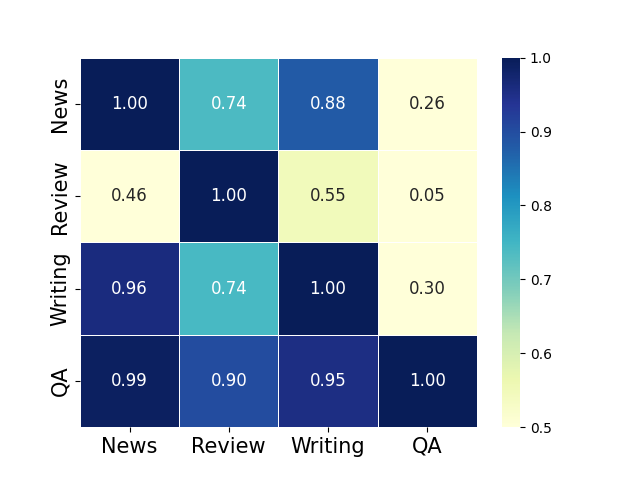}
\end{minipage}
}
\subfloat[\footnotesize 1 - FPR]
{\label{fig:ad3}
\begin{minipage}[b]{0.24\linewidth}
\centering
\includegraphics[width=1.1\textwidth]{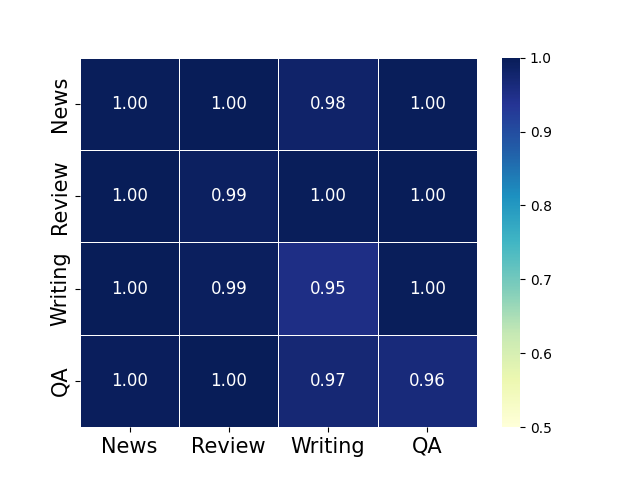}
\end{minipage}
}
\caption{\small Generalization \& MAUVE across Various Domains with all Human}
\label{fig:topic_similar5}
\end{figure}

% \textbf{Detectors without Training.} The impact of prompts in evaluation (for methods without training involved). 
% \begin{table*}[h!]
% \centering
% \caption{ChatGPT Detection Performance (True Positive Rate)}
% \label{tab:indistribution}
% \resizebox{0.7\textwidth}{!}
% {
% \begin{tabular}{c|| ccc | ccc | ccc | ccc  } 
% \hline
% \hline
% & \multicolumn{3}{c|}{News} &  \multicolumn{3}{c|}{Review} & \multicolumn{3}{c|}{Writing} & \multicolumn{3}{c}{QA} \\
%  & p1 & p2 & p3  & p1 & p2 & p3  & p1 & p2 & p3  & p1 & p2 & p3 \\
% \hline
% GPTZero & 1.00 & 1.00 & 1.00 & 0.92 & 0.72 & 0.87 & 1.00 & 1.00 & 0.91 & 0.98 & 0.97 &  0.98\\
% DNA-GPT & 0.95 & 0.88 & 0.83 & 0.90 & 0.94 & 0.83 & 0.99 & 1.00 & 0.78 & 0.95 & 0.77 & 0.88\\
% \hline\hline
% \end{tabular}
% }
% \end{table*}
